# Supplementary material for: On the Analysis of Spatially Constrained Power of Two Choice Policies
Source: arXiv:2011.02653 source file (2020-11-05)
Supplement: Supplementary file 1 [file 06-appendix.tex]

Our goal is to study the distributions of load and request distance under various randomized load balancing policies in a spatial setting. We simulate a large system with $2n$ nodes randomly (uniformly) distributed in a unit square, where $n=50,000$. %Nodes $\{1,2,\ldots,n\}$ are users and $\{n+1,\ldots,n\}$ are servers. 
We perform a single simulation run and measure the distributions of load across all the servers and of the request distance to the chosen server. 

First we focus on the server loads in Figure \ref{fig:loadplots}. Obviously the sPOO policy performs the worst and sPOT performs somewhat better, but the latter does not provide the ``power-of-two" benefit (corroborates our previous result).  

Not surprisingly, the sPOO and sPOT policies perform really well in terms of request distance as evidenced from Figure \ref{fig:distplots}, but this comes at the cost of highly imbalanced loads.

Finally, the dPOT policies achieve the best of both worlds, i.e., low maximum load and low distances because they significantly favor closer nodes. dPOT has no visible difference in load performance as compared to POT as shown in  Figures \ref{fig:loadplots}. dPOT policy performs better than POT in terms of distance distributions as evidenced in the plots in Figure \ref{fig:distplots}\footnote{Note that since the $X$ values span a narrow range, the PDF values can exceed 1 on the $Y$-axis, sometimes significantly. These are valid PDFs with area under curve equal to 1.}.
